# Supplementary material for: Energy Transfer into Period-Tripled States in Coupled Electromechanical Modes at Internal Resonance
Source: arXiv:2206.01630 source file (2022-09-20)
Supplement: Supplementary file 1 [file yan_supplementary.pdf]

# Supplementary material of “Energy Transfer into Period-Tripled States in Coupled Electromechanical Modes at Internal Resonance”

Yingming Yan,[1,2] X. Dong,[1,2] L. Huang,[1,2] K. Moskovtsev[3] and H. B. Chan[1,2]

[1]Department of Physics, The Hong Kong University of Science and Technology, Hong Kong, China
[2]William Mong Institute of Nano Science and Technology, The Hong Kong University of Science and Technology, Clear Water Bay, Kowloon, Hong Kong, China

[3]Department of Physics and Astronomy, Michigan State University, East Lansing, Michigan 48824, USA

## A. Finite element modeling and measurement of other vibrational modes

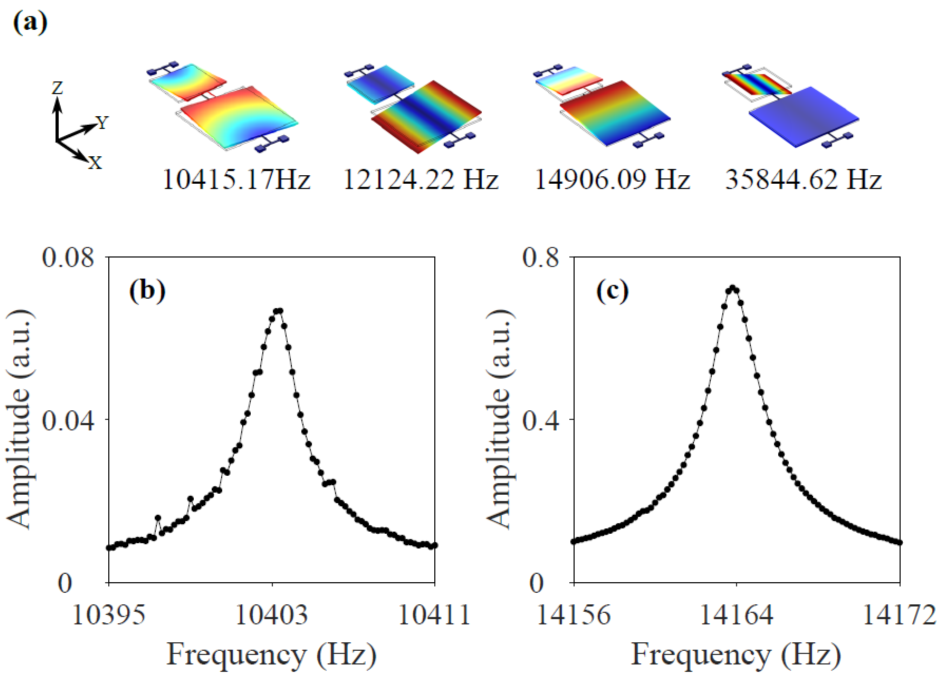


FIG. S. 1. (a) The vibrational profiles of the first four vibrational modes calculated using finite element analysis (COMSOL). The second and fourth modes correspond to modes 1 and 2 in the main text respectively. For the first mode, the beams are deformed in the x-y direction and the two plates vibrate parallel to the substrate. For the third mode, the beams are deformed so that displacements are in the x and z directions only. Measured resonant response of the modes with (b) the lowest frequency and (c) the third lowest energy.

The vibrational modes of our device are modelled using finite element analysis (COMSOL). Figure S. 1 shows the results for the first four modes. The second and fourth modes are torsional modes. They correspond to modes 1 and 2 in the main text respectively. Their eigenfrequencies are designed to be close to a ratio of 1:3 so that they can be tuned into internal resonance by applying voltages to the electrodes.

The other two modes can also be observed in measurement. Figures S. 1(b) and (c) plot the measured response of the large plate for the modes with the lowest and the third lowest frequency respectively when periodic voltages near their resonant frequencies are applied to the electrodes. Their role in the present study is negligible because they do not yield integer ratios of resonant frequencies with modes 1 and 2. The resonant linewidths of all the modes shown in Fig. S. 1 are narrow (several Hz) compared to the eigenfrequencies (> 10 kHz). To further check the validity of our theoretical analysis that only uses modes 1 and 2, we measure the other modes when vibrations of modes 1 and 2 are excited in the period-tripled regime. We find no detectable response in the other modes.

## B. Linear friction in modes 1 and 2

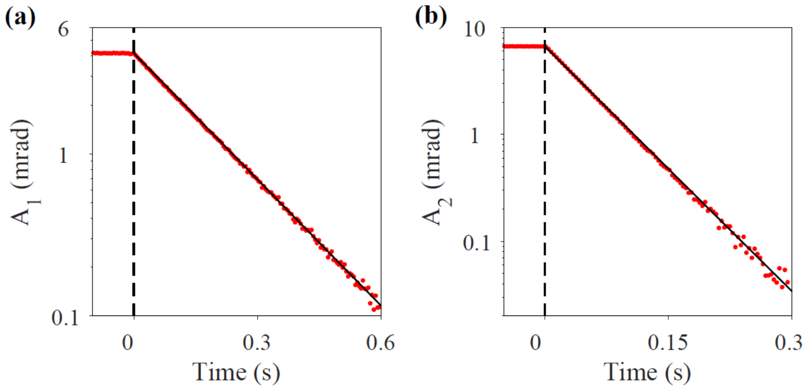


FIG. S. 2. Measured vibration amplitude (circles) of (a) mode 1 and (b) mode 2 on a semi-logarithmic scale as a function of time. The resonant drives on the modes are removed at time t = 0 s, marked by the dashed lines. The solid lines are fits of exponential decay. The frequency mismatch of the two modes is $\varepsilon_1/2\pi$ = 10 Hz.

When the periodic drives to mode 1 and mode 2 are removed, the amplitude of vibrations decays. Figure S. 2(a) shows measurement of the ring down of vibrations of mode 1. The mode is resonantly driven into vibrations, at an amplitude comparable to those for period-tripled vibrations described in the main text. When the drive is removed at time t = 0 s, the amplitude of vibrations decays exponentially. Figure S. 2(b) shows similar measurement for mode 2. These ringdown measurements indicate that energy dissipation in our system is dominated by linear friction. It is not necessary to explicitly include nonlinear friction terms that depend on vibration amplitude in the equation of motion.

Due to the Duffing nonlinearity, the eigenfrequency of each mode increases as the vibration amplitude decreases. In Fig. S. 2, the frequency mismatch $\varepsilon_1 = \omega_2/3 - \omega_1$ is chosen to ensure that the ratio of the eigenfrequencies never gets close to 3 for internal resonance and there is no energy exchange between two modes. For other choices of $\varepsilon_1$ that allow the system to enter into the regime of internal resonance during the ringdown, the interaction energy $\gamma q_1^3 q_2$ can give rise to decay coefficients dependent on the vibration amplitude. Such nonlinear damping has been observed by a number of groups [s1, s2].

## C. Contributions of geometric nonlinearity to the coupling energy

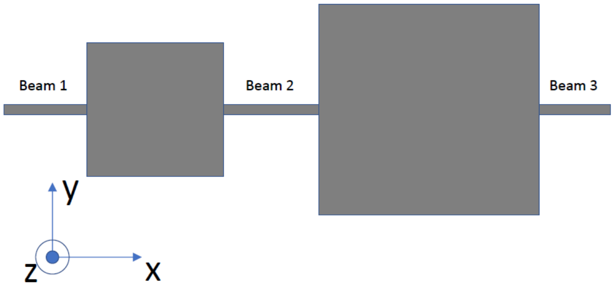


FIG. S. 3. Device dimensions used in calculating the contributions of geometric nonlinearity to the coupling energy (Not to scale).

There are three torsional beams in our device, labelled as beams 1, 2 and 3 in Fig. S. 3. Beams 1 and 3 are assumed to be identical. The torsional spring constants $k_j$ ($j$ = 1, 2, 3) are given by:

$$k_j = \frac{2 l_{jy}^4 c_{44}}{3 l_{jx}}, \qquad \text{(S1)}$$

where $c_{44}$ is the shear elastic constant, $l_{jx}$ and $l_{jy}$ are the length and the width of beam $j$ respectively. The beams are assumed to have square cross-sections. We denote the angular displacements of the two plates from their rest positions by $\phi_{1,2}$. For small $\phi_{1,2}$, the equations of motion are given by:

$$I_1 \ddot{\phi}_1 = -(k_1 + k_2)\phi_1 + k_2 \phi_2$$

$$I_2 \ddot{\phi}_2 = -(k_2 + k_3)\phi_2 + k_2 \phi_1. \qquad \text{(S2)}$$

Modes 1 and 2 described in the main text are the normal modes, with frequencies given by:

$$\omega_{1,2}^2 = \frac{1}{2I_1I_2}\left[I_2(k_1+k_2)+I_2(k_2+k_3) \pm \sqrt{[I_2(k_1+k_2)-I_1(k_2+k_3)]^2+4I_1I_2k_2^2}\,\right]. \quad \text{(S3)}$$

For mode *i* (*i* = 1, 2), the ratio $\xi_i$ of the angles of the two plates can be determined from Eq. (S2). When the system vibrates in mode *i* with amplitude $Q_i$, the angles of plates 1 and 2 are given by $\phi_1^{(i)} = \beta_i Q_i$ and $\phi_2^{(i)} = \xi_i \beta_i Q_i$ respectively, where $\beta_i$ is a normalization constant.

Beam 1 is fixed at its left end. When the right end is rotated by angle θ about the x axis, the displacement vector at point (*x*, *y*, *z*) is:

$$u_x = 0$$

$$u_y = y\left[\cos\left({\theta x}/{l_x}\right) - 1\right] - z\sin({\theta x}/{l_x})$$

$$u_z = y\sin({\theta x}/{l_x}) + z\left[\cos\left({\theta x}/{l_x}\right) - 1\right]. \quad \text{(S4)}$$

This displacement field gives the Lagrangian strain field:

$$\varepsilon_1 \equiv \varepsilon_{xx} = \frac{\theta^2}{2l_x^2}(y^2+z^2)$$

$$\varepsilon_5 \equiv 2\varepsilon_{xz} = \theta y/l_x$$

$$\varepsilon_6 \equiv 2\varepsilon_{xy} = -\theta z/l_x. \quad \text{(S5)}$$

$\theta$ contains contributions from both modes. The strains for beams 2 and 3 can also be calculated using a similar procedure.

The elastic potential energy is then calculated with

$$F = \int d\boldsymbol{r}\,\frac{1}{2}c_{IJ}\,\varepsilon_I\varepsilon_J, \quad \text{(S6)}$$

where $c_{ij}$ are the second order stiffness tensor. Contributions due to material nonlinearities are assumed to be negligible.

From Eq. (S6), we identify the coupling energy of the form $Q_1^3 Q_2 \beta_1^3 \beta_2 U_c$ due to geometrical nonlinearity, where $U_c$ is given by:

$$U_c = \frac{0.019\xi_2}{l_{2x}^3}\xi_1^3 c_{11} l_{2y}^6 + \frac{0.019\xi_2}{l_{1x}^3}\xi_1^3 c_{11} l_{1y}^6 - \frac{0.019c_{11}}{l_{2x}^3}\xi_1^3 l_{2y}^6 - \frac{0.06\xi_2}{l_{2x}^3}\xi_1^2 c_{11} l_{2y}^6 + \frac{0.058c_{11}}{l_{2x}^3}\xi_1^2 l_{2y}^6 +$$
$$\frac{0.058\xi_1}{l_{2x}^3}\xi_2 c_{11} l_{2y}^6 - \frac{0.058\xi_1}{l_{2x}^3} c_{11} l_{2y}^6 - \frac{0.019\xi_2}{l_{2x}^3} c_{11} l_{2y}^6 + \frac{0.019c_{11}}{l_{2x}^3} l_{2y}^6 + \frac{0.019c_{11}}{l_{1x}^3} l_{1y}^6. \quad \text{(S7)}$$

All terms in the expression have a similar structure: $\propto c_{IJ} l_{jy}^6 / l_{jx}^3$. In the experiment, the dimensions of the torsional rods are chosen to maximize this coupling, while keeping the spring constants sufficiently small so that vibrations can be induced with small voltages to the electrodes.


[s1] C. Chen, D. H. Zanette, D. A. Czaplewski, S. Shaw and D. Lopez, *Direct observation of coherent energy transfer in nonlinear micromechanical oscillators*, Nature Communications **8**, 15523 (2017).

[s2] J. Guttinger, A. Noury, P. Weber, A. M. Eriksson, C. Lagoin, J. Moser, C. Eichler, A. Wallraff, A. Isacsson and A. Bachtold, *Energy-dependent path of dissipation in nanomechanical resonators*, Nature Nanotechnology **12**, 631 (2017).
